# Supplementary material for: GPU Methodologies for Numerical Partial Differential Equations
Source: arXiv:2101.06550 source file (2021-01-16)
Supplement: Supplementary file 1 [file AppendixA.tex]

\chapter{Perturbation expansion of the detuned triad}
\label{appdx:detunedtriad}
