# Supplementary material for: GPU Methodologies for Numerical Partial Differential Equations
Source: arXiv:2101.06550 source file (2021-01-16)
Supplement: Supplementary file 2 [file AppendixB.tex]

\chapter{Integrating the detuned triad equations}
\label{appdx:triadinteg}
