# Supplementary material for: GPU Methodologies for Numerical Partial Differential Equations
Source: arXiv:2101.06550 source file (2021-01-16)
Supplement: Supplementary file 3 [file AppendixC.tex]

\chapter{Coefficients of the quasi-resonant five-wave equations in phase-amplitude form}
\label{appdx:5wavecoeff}
